# Supplementary material for: EBDM: Exemplar-guided Image Translation with Brownian-bridge Diffusion Models
Source: arXiv:2410.09802 source file (2024-10-13)
Supplement: Supplementary file 3 [file 3_experiments.tex]

\pagebreak
\section{User Study.}
We conducted a user study to evaluate the quality of the generated images. We randomly selected 100 images from the test set and asked 00 participants to compare the images generated by EBDM with those generated by LDM and BBDM. The participants were asked to choose the better image between the two images. The results are shown in Table 0. The results show that EBDM outperforms LDM and BBDM in terms of image quality.
