# Supplementary material for: EBDM: Exemplar-guided Image Translation with Brownian-bridge Diffusion Models
Source: arXiv:2410.09802 source file (2024-10-13)
Supplement: Supplementary file 4 [file tab2.tex]

\begin{table*}
    % \resizebox{\textwidth}{!}{
      \centering
    \begin{tabular}{ccccc}
    \hline
        model &
        start step &
        \makecell{decay} &
        \makecell{update interval} &
        \makecell{batch size} \\
        \hline
        EBDM-f4 & 30000 & 0.995 & 16 & 8 \\
        EBDM-f8 & 30000 & 0.995 & 16 & 8 \\
        EBDM-f16 & 15000 & 0.995 & 8 & 16 \\
        \hline
    \end{tabular}
    % }
    \caption{EMA hyperparameters of EBDM.}
    \label{tab:sup2}
    \end{table*}
