# Supplementary material for: EBDM: Exemplar-guided Image Translation with Brownian-bridge Diffusion Models
Source: arXiv:2410.09802 source file (2024-10-13)
Supplement: Supplementary file 5 [file tab3.tex]

\begin{table*}[bt!]
      \centering
    \begin{tabular}{ccccccc}
    \hline
        model &
        max learning rate & min learning rate & factor & patience & cool down & threshold \\
        \hline
        EBDM-f4 & $1.0 \mathrm{e}-4$ & $5.0 \mathrm{e}-7$ & 0.5 & 3000 & 2000 & $1.0 \mathrm{e}-4$ \\
        EBDM-f8 & $1.0 \mathrm{e}-4$ & $5.0 \mathrm{e}-7$ & 0.5 & 3000 & 2000 & $1.0 \mathrm{e}-4$ \\
        EBDM-f16 & $1.0 \mathrm{e}-4$ & $1.0 \mathrm{e}-6$ & 0.5 & 3000 & 2000 & $1.0 \mathrm{e}-4$ \\
        \hline
    \end{tabular}
    % }
    \caption{Learning rate scheduler hyperparameters of BBDM.}
    \label{tab:sup3}
\end{table*}
